# Supplementary material for: Symbolic inductive bias for visually grounded learning of spoken language
Source: arXiv:1812.09244 source file (2019-06-05)
Supplement: Supplementary file 1 [file appendix.tex]

\begin{appendices}

\section{Detailed results}
\begin{table*}
\begin{tabular}{llrrrrrrrr}\toprule
Model   &       Data       & Symbol & epoch & R@1    & R@5   & R@10   & medr    &  RSA    & Speaker     \\\midrule
Baseline  & -              & char   & 24    & 0.04   & 0.15  & 0.23   & 58.0    &  0.18   & 0.31  \\ % green:libri-audiotext-3a
Baseline  & -              & char   & 18    & 0.04   & 0.15  & 0.23   & 58.0    &  0.19   & 0.30  \\ % cartesius: libri-audiotext-3
Transcription & -          & char   & 21    & 0.08   & 0.27  & 0.38   & 20.0    &  0.27   & NA    \\ %  green:transcription-4
\if False
Shared-4  & disjoint       & char   & 25    & 0.02   & 0.09  & 0.14   & 96.0    &  0.19   & 0.31  \\ %  green:libri-audiotext-2
Shared-4  & disjoint       & char   & 23    & 0.02   & 0.09  & 0.15   & 89.0    &  0.19   & 0.29  \\ %  cartesius: libri-audiotext-5
Shared-2-T2,2  & disjoint  & char   & 24    & 0.03   & 0.12  & 0.21   & 65.0    &  0.21   & 0.27  \\ % green: libri-audiotext-partial-2
Shared-2-T1,2  & disjoint  & char   & 24    & 0.05   & 0.17  & 0.25   & 50.0    &  0.21   & 0.22  \\ % green: libri-audiotext-partial-3
Shared-2-T0,2  & disjoint  & char   & 23    & 0.05   & 0.17  & 0.27   & 46.5    &  0.21   & 0.18  \\ % green: libri-audiotext-partial-4
Shared-2-T0,2  & disjoint  & char   & 23    & 0.05   & 0.18  & 0.27   & 45.0    &  0.21   & 0.17  \\ % cartesius: shared-2-t0,2-disjoint
Shared-3-T0,2  & disjoint  & char   & 24    & 0.04   & 0.14  & 0.22   & 61.0    &  0.20   & 0.22  \\ % green: shared-3-T0,2-disjoint
Shared-2-T0,1  & disjoint  & char   & 24    & 0.05   & 0.17  & 0.27   & 45.0    &  0.21   & 0.18  \\ % green: shared-2-t0,1-disjoint
Shared-1-T1,2  & disjoint  & char   & 25    & 0.05   & 0.17  & 0.25   & 51.0    &  0.20   & 0.20  \\ % green: shared-1-t1,2-disjoint
Shared-0-T2,2  & disjoint  & char   & 24    & 0.04   & 0.16  &  0.25  & 54.0    &  0.20   & 0.24  \\ % green: shared-0-t2,2-disjoint
Shared-2-T0,1 & disjoint   & word   & 24    & 0.04   & 0.17  & 0.25   & 52.0    &  0.21   & 0.25 \\ % green: word-shared-2-t0,1-disjoint
Shared-1-T0,1 & disjoint   & word   & 23    & 0.05   & 0.17  & 0.26   & 48.0    &  0.22   & 0.23 \\ % green: word-shared-1-t0,1-disjoint 
Shared-1-T0,2 & disjoint   & word   & 24    & 0.05   & 0.17  & 0.25   & 51.0    &  0.21   & 0.23 \\ % green: word-shared-1-t0,2-disjoint
Shared-1-T1,1 & disjoint   & word   & 23    & 0.05   & 0.16  & 0.24   & 55.0    &  0.21   & 0.25 \\ % green: word-shared-1-t1,1-disjoint
\midrule
Shared-2-T1,2  & joint     & char   & 19    & 0.05   & 0.18  & 0.27   & 46.0    &  0.22   & 0.19  \\ % green: flickr-audiotext-partial-1
Shared-2-T0,2  & joint     & char   & 24    & 0.05   & 0.18  & 0.27   & 46.0    &  0.21   & 0.09  \\ % green: flickr-audiotext-partial-2
Shared-2-T0,2  & joint     & char   & 22    & 0.05   & 0.17  & 0.27   & 44.0    &  0.21   & 0.11  \\ % cartesius: shared-2-t0,2-joint
Shared-2-T0,1  & joint     & char   & 23    & 0.05   & 0.18  & 0.27   & 43.0    &  0.22   & 0.09   \\ % green: flickr-audiotext-partial-3
\midrule
\fi
3way-s2-si2 &  & char   & 22    &  0.03   &  0.13  &  0.20  &  72.50    &  0.18    &  0.29  \\% green:3way-s2-si2--e
3way-s2-si2 &  & char   & 24    &  0.04   &  0.15  &  0.24  &  60.00    &  0.19    &  0.33  \\% green:3way-s2-si2--f
3way-s2-si2 &  & char   & 19    &  0.04   &  0.15  &  0.22  &  59.00    &  0.19    &  0.27  \\% green:3way-s2-si2--g

3way-s2-t1-st0-si2 & joint & char   & 23    &  0.06   &  0.19  &  0.28  &  41.00    &  0.21    &  0.10  \\% green:3way-s2-t1-st0-si2-joint-e
3way-s2-t1-st0-si2 & joint & char   & 25    &  0.05   &  0.19  &  0.28  &  43.00    &  0.21    &  0.11  \\% green:3way-s2-t1-st0-si2-joint-f
3way-s2-t1-st0-si2 & joint & char   & 21    &  0.05   &  0.18  &  0.27  &  43.00    &  0.22    &  0.10  \\% green:3way-s2-t1-st0-si2-joint-g

3way-s2-t1-st0-si2-ti1 & joint & char   & 19    &  0.06   &  0.19  &  0.28  &  39.00    &  0.22    &  0.08  \\% green:3way-s2-t1-st0-si2-ti1-joint-e
3way-s2-t1-st0-si2-ti1 & joint & char   & 24    &  0.05   &  0.20  &  0.29  &  38.00    &  0.22    &  0.09  \\% green:3way-s2-t1-st0-si2-ti1-joint-f
3way-s2-t1-st0-si2-ti1 & joint & char   & 22    &  0.06   &  0.18  &  0.28  &  42.00    &  0.22    &  0.08  \\% green:3way-s2-t1-st0-si2-ti1-joint-g
3way-s2-t1-st1,1-si2-ti1 & joint & char   & 25    &  0.05   &  0.18  &  0.27  &  46.00    &  0.21    &  0.16  \\% green:3way-s2-t1-st1,1-si2-ti1-joint-e
3way-s2-t1-st1,1-si2-ti1 & joint & char   & 22    &  0.05   &  0.18  &  0.27  &  44.00    &  0.21    &  0.17  \\% green:3way-s2-t1-st1,1-si2-ti1-joint-f
3way-s2-t1-st1,1-si2-ti1 & joint & char   & 25    &  0.05   &  0.18  &  0.27  &  43.00    &  0.21    &  0.17  \\% green:3way-s2-t1-st1,1-si2-ti1-joint-g
3way-s3-t2-st0-si2-ti1 & joint & char   & 20    &  0.05   &  0.16  &  0.25  &  50.00    &  0.22    &  0.07  \\% green:3way-s3-t2-st0-si2-ti1-joint-e
3way-s3-t2-st0-si2-ti1 & joint & char   & 25    &  0.05   &  0.17  &  0.26  &  50.00    &  0.22    &  0.07  \\% green:3way-s3-t2-st0-si2-ti1-joint-f
3way-s2-t1-st0-si1-ti1 & joint & char   & 21    &  0.05   &  0.18  &  0.28  &  43.00    &  0.22    &  0.24  \\% green:3way-s2-t1-st0-si1-ti1-joint-e
3way-s2-t1-st0-si1-ti1 & joint & char   & 25    &  0.05   &  0.19  &  0.28  &  44.00    &  0.21    &  0.23  \\% green:3way-s2-t1-st0-si1-ti1-joint-f
3way-s2-t1-st0-si1-ti1 & joint & char   & 24    &  0.05   &  0.19  &  0.28  &  42.00    &  0.20    &  0.25  \\% green:3way-s2-t1-st0-si1-ti1-joint-g

3way-s2-t1-st0-si2 & disjoint & char   & 25    &  0.05   &  0.18  &  0.27  &  44.00    &  0.21    &  0.18  \\% green:3way-s2-t1-st0-si2-disjoint-e
3way-s2-t1-st0-si2 & disjoint & char   & 20    &  0.06   &  0.19  &  0.28  &  40.00    &  0.22    &  0.16  \\% green:3way-s2-t1-st0-si2-disjoint-f
3way-s2-t1-st0-si2 & disjoint & char   & 24    &  0.05   &  0.19  &  0.28  &  40.00    &  0.22    &  0.18  \\% green:3way-s2-t1-st0-si2-disjoint-g

3way-s2-t1-st0-si2-ti1 & disjoint & char   & 24    &  0.05   &  0.18  &  0.28  &  42.00    &  0.22    &  0.18  \\% green:3way-s2-t1-st0-si2-ti1-disjoint-e
3way-s2-t1-st0-si2-ti1 & disjoint & char   & 21    &  0.05   &  0.19  &  0.28  &  40.00    &  0.22    &  0.19  \\% green:3way-s2-t1-st0-si2-ti1-disjoint-f
3way-s2-t1-st0-si2-ti1 & disjoint & char   & 25    &  0.05   &  0.18  &  0.28  &  43.00    &  0.20    &  0.17  \\% green:3way-s2-t1-st0-si2-ti1-disjoint-g

3way-s2-t1-st0-si2-ti1-tr0,1 & joint & char   & 20    &  0.06   &  0.20  &  0.29  &  40.00    &  0.22    &  0.09  \\% green:3way-s2-t1-st0-si2-ti1-tr0,1-joint-e
3way-s2-t1-st0-si2-ti1-tr0,1 & joint & char   & 19    &  0.06   &  0.20  &  0.30  &  36.50    &  0.22    &  0.08  \\% green:3way-s2-t1-st0-si2-ti1-tr0,1-joint-f
3way-s2-t1-st0-si2-ti1-tr0,1 & joint & char   & 24    &  0.06   &  0.21  &  0.30  &  38.00    &  0.22    &  0.09  \\% green:3way-s2-t1-st0-si2-ti1-tr0,1-joint-g

\midrule

\bottomrule
\end{tabular}
\end{table*}
\end{appendices}
